# Supplementary material for: RIDE: Self-Supervised Learning of Rotation-Equivariant Keypoint Detection and Invariant Description for Endoscopy
Source: arXiv:2309.09563 source file (2023-09-18)
Supplement: Supplementary file 1 [file supp.tex]

%%%%%%%%%%%%%%%%%%%%%%%%%%%%%%%%%%%%%%%%%%%%%%%%%%%%%%%%%%%%%%%%%%%%%%%%%%%%%%%%
%2345678901234567890123456789012345678901234567890123456789012345678901234567890
%        1         2         3         4         5         6         7         8

\documentclass[letterpaper, 10 pt, conference]{ieeeconf}  % Comment this line out if you need a4paper

\IEEEoverridecommandlockouts                              % This command is only needed if 
                                                          % you want to use the \thanks command

\overrideIEEEmargins                                      % Needed to meet printer requirements.

%In case you encounter the following error:
%Error 1010 The PDF file may be corrupt (unable to open PDF file) OR
%Error 1000 An error occurred while parsing a contents stream. Unable to analyze the PDF file.
%This is a known problem with pdfLaTeX conversion filter. The file cannot be opened with acrobat reader
%Please use one of the alternatives below to circumvent this error by uncommenting one or the other
%\pdfobjcompresslevel=0
%\pdfminorversion=4

% See the \addtolength command later in the file to balance the column lengths
% on the last page of the document

% The following packages can be found on http:\\www.ctan.org
%\usepackage{graphics} % for pdf, bitmapped graphics files
%\usepackage{epsfig} % for postscript graphics files
%\usepackage{mathptmx} % assumes new font selection scheme installed
%\usepackage{times} % assumes new font selection scheme installed
%\usepackage{amsmath} % assumes amsmath package installed
%\usepackage{amssymb}  % assumes amsmath package installed

\title{\LARGE \bf
Preparation of Papers for IEEE Sponsored Conferences \& Symposia*
}

\author{Albert Author$^{1}$ and Bernard D. Researcher$^{2}$% <-this % stops a space
\thanks{*This work was not supported by any organization}% <-this % stops a space
\thanks{$^{1}$Albert Author is with Faculty of Electrical Engineering, Mathematics and Computer Science,
        University of Twente, 7500 AE Enschede, The Netherlands
        {\tt\small albert.author@papercept.net}}%
\thanks{$^{2}$Bernard D. Researcheris with the Department of Electrical Engineering, Wright State University,
        Dayton, OH 45435, USA
        {\tt\small b.d.researcher@ieee.org}}%
}

\begin{document}

\maketitle
\thispagestyle{empty}
\pagestyle{empty}

%%%%%%%%%%%%%%%%%%%%%%%%%%%%%%%%%%%%%%%%%%%%%%%%%%%%%%%%%%%%%%%%%%%%%%%%%%%%%%%%
\begin{abstract}

This electronic document is a ÒliveÓ template. The various components of your paper [title, text, heads, etc.] are already defined on the style sheet, as illustrated by the portions given in this document.

\end{abstract}

%%%%%%%%%%%%%%%%%%%%%%%%%%%%%%%%%%%%%%%%%%%%%%%%%%%%%%%%%%%%%%%%%%%%%%%%%%%%%%%%
\section{INTRODUCTION}

This template provides authors with most of the formatting specifications needed for preparing electronic versions of their papers. All standard paper components have been specified for three reasons: (1) ease of use when formatting individual papers, (2) automatic compliance to electronic requirements that facilitate the concurrent or later production of electronic products, and (3) conformity of style throughout a conference proceedings. Margins, column widths, line spacing, and type styles are built-in; examples of the type styles are provided throughout this document and are identified in italic type, within parentheses, following the example. Some components, such as multi-leveled equations, graphics, and tables are not prescribed, although the various table text styles are provided. The formatter will need to create these components, incorporating the applicable criteria that follow.

\section{PROCEDURE FOR PAPER SUBMISSION}

\subsection{Selecting a Template (Heading 2)}

First, confirm that you have the correct template for your paper size. This template has been tailored for output on the US-letter paper size. 
It may be used for A4 paper size if the paper size setting is suitably modified.

\subsection{Maintaining the Integrity of the Specifications}

The template is used to format your paper and style the text. All margins, column widths, line spaces, and text fonts are prescribed; please do not alter them. You may note peculiarities. For example, the head margin in this template measures proportionately more than is customary. This measurement and others are deliberate, using specifications that anticipate your paper as one part of the entire proceedings, and not as an independent document. Please do not revise any of the current designations

\section{MATH}

Before you begin to format your paper, first write and save the content as a separate text file. Keep your text and graphic files separate until after the text has been formatted and styled. Do not use hard tabs, and limit use of hard returns to only one return at the end of a paragraph. Do not add any kind of pagination anywhere in the paper. Do not number text heads-the template will do that for you.

Finally, complete content and organizational editing before formatting. Please take note of the following items when proofreading spelling and grammar:

\subsection{Abbreviations and Acronyms} Define abbreviations and acronyms the first time they are used in the text, even after they have been defined in the abstract. Abbreviations such as IEEE, SI, MKS, CGS, sc, dc, and rms do not have to be defined. Do not use abbreviations in the title or heads unless they are unavoidable.

\subsection{Units}

\begin{itemize}

\item Use either SI (MKS) or CGS as primary units. (SI units are encouraged.) English units may be used as secondary units (in parentheses). An exception would be the use of English units as identifiers in trade, such as Ò3.5-inch disk driveÓ.
\item Avoid combining SI and CGS units, such as current in amperes and magnetic field in oersteds. This often leads to confusion because equations do not balance dimensionally. If you must use mixed units, clearly state the units for each quantity that you use in an equation.
\item Do not mix complete spellings and abbreviations of units: ÒWb/m2Ó or Òwebers per square meterÓ, not Òwebers/m2Ó.  Spell out units when they appear in text: Ò. . . a few henriesÓ, not Ò. . . a few HÓ.
\item Use a zero before decimal points: Ò0.25Ó, not Ò.25Ó. Use Òcm3Ó, not ÒccÓ. (bullet list)

\end{itemize}

\subsection{Equations}

The equations are an exception to the prescribed specifications of this template. You will need to determine whether or not your equation should be typed using either the Times New Roman or the Symbol font (please no other font). To create multileveled equations, it may be necessary to treat the equation as a graphic and insert it into the text after your paper is styled. Number equations consecutively. Equation numbers, within parentheses, are to position flush right, as in (1), using a right tab stop. To make your equations more compact, you may use the solidus ( / ), the exp function, or appropriate exponents. Italicize Roman symbols for quantities and variables, but not Greek symbols. Use a long dash rather than a hyphen for a minus sign. Punctuate equations with commas or periods when they are part of a sentence, as in

$$
\alpha + \beta = \chi \eqno{(1)}
$$

Note that the equation is centered using a center tab stop. Be sure that the symbols in your equation have been defined before or immediately following the equation. Use Ò(1)Ó, not ÒEq. (1)Ó or Òequation (1)Ó, except at the beginning of a sentence: ÒEquation (1) is . . .Ó

\subsection{Some Common Mistakes}
\begin{itemize}

\item The word ÒdataÓ is plural, not singular.
\item The subscript for the permeability of vacuum ?0, and other common scientific constants, is zero with subscript formatting, not a lowercase letter ÒoÓ.
\item In American English, commas, semi-/colons, periods, question and exclamation marks are located within quotation marks only when a complete thought or name is cited, such as a title or full quotation. When quotation marks are used, instead of a bold or italic typeface, to highlight a word or phrase, punctuation should appear outside of the quotation marks. A parenthetical phrase or statement at the end of a sentence is punctuated outside of the closing parenthesis (like this). (A parenthetical sentence is punctuated within the parentheses.)
\item A graph within a graph is an ÒinsetÓ, not an ÒinsertÓ. The word alternatively is preferred to the word ÒalternatelyÓ (unless you really mean something that alternates).
\item Do not use the word ÒessentiallyÓ to mean ÒapproximatelyÓ or ÒeffectivelyÓ.
\item In your paper title, if the words Òthat usesÓ can accurately replace the word ÒusingÓ, capitalize the ÒuÓ; if not, keep using lower-cased.
\item Be aware of the different meanings of the homophones ÒaffectÓ and ÒeffectÓ, ÒcomplementÓ and ÒcomplimentÓ, ÒdiscreetÓ and ÒdiscreteÓ, ÒprincipalÓ and ÒprincipleÓ.
\item Do not confuse ÒimplyÓ and ÒinferÓ.
\item The prefix ÒnonÓ is not a word; it should be joined to the word it modifies, usually without a hyphen.
\item There is no period after the ÒetÓ in the Latin abbreviation Òet al.Ó.
\item The abbreviation Òi.e.Ó means Òthat isÓ, and the abbreviation Òe.g.Ó means Òfor exampleÓ.

\end{itemize}

\section{USING THE TEMPLATE}

Use this sample document as your LaTeX source file to create your document. Save this file as {\bf root.tex}. You have to make sure to use the cls file that came with this distribution. If you use a different style file, you cannot expect to get required margins. Note also that when you are creating your out PDF file, the source file is only part of the equation. {\it Your \TeX\ $\rightarrow$ PDF filter determines the output file size. Even if you make all the specifications to output a letter file in the source - if your filter is set to produce A4, you will only get A4 output. }

It is impossible to account for all possible situation, one would encounter using \TeX. If you are using multiple \TeX\ files you must make sure that the ``MAIN`` source file is called root.tex - this is particularly important if your conference is using PaperPlaza's built in \TeX\ to PDF conversion tool.

\subsection{Headings, etc}

Text heads organize the topics on a relational, hierarchical basis. For example, the paper title is the primary text head because all subsequent material relates and elaborates on this one topic. If there are two or more sub-topics, the next level head (uppercase Roman numerals) should be used and, conversely, if there are not at least two sub-topics, then no subheads should be introduced. Styles named ÒHeading 1Ó, ÒHeading 2Ó, ÒHeading 3Ó, and ÒHeading 4Ó are prescribed.

\subsection{Figures and Tables}

Positioning Figures and Tables: Place figures and tables at the top and bottom of columns. Avoid placing them in the middle of columns. Large figures and tables may span across both columns. Figure captions should be below the figures; table heads should appear above the tables. Insert figures and tables after they are cited in the text. Use the abbreviation ÒFig. 1Ó, even at the beginning of a sentence.

\begin{table}[h]
\caption{An Example of a Table}
\label{table_example}
\begin{center}
\begin{tabular}{|c||c|}
\hline
One & Two\\
\hline
Three & Four\\
\hline
\end{tabular}
\end{center}
\end{table}

   \begin{figure}[thpb]
      \centering
      \framebox{\parbox{3in}{We suggest that you use a text box to insert a graphic (which is ideally a 300 dpi TIFF or EPS file, with all fonts embedded) because, in an document, this method is somewhat more stable than directly inserting a picture.
}}
      \caption{Inductance of oscillation winding on amorphous
       magnetic core versus DC bias magnetic field}
      \label{figurelabel}
   \end{figure}

Figure Labels: Use 8 point Times New Roman for Figure labels. Use words rather than symbols or abbreviations when writing Figure axis labels to avoid confusing the reader. As an example, write the quantity ÒMagnetizationÓ, or ÒMagnetization, MÓ, not just ÒMÓ. If including units in the label, present them within parentheses. Do not label axes only with units. In the example, write ÒMagnetization (A/m)Ó or ÒMagnetization {A[m(1)]}Ó, not just ÒA/mÓ. Do not label axes with a ratio of quantities and units. For example, write ÒTemperature (K)Ó, not ÒTemperature/K.Ó

\section{CONCLUSIONS}

A conclusion section is not required. Although a conclusion may review the main points of the paper, do not replicate the abstract as the conclusion. A conclusion might elaborate on the importance of the work or suggest applications and extensions. 

\addtolength{\textheight}{-12cm}   % This command serves to balance the column lengths
                                  % on the last page of the document manually. It shortens
                                  % the textheight of the last page by a suitable amount.
                                  % This command does not take effect until the next page
                                  % so it should come on the page before the last. Make
                                  % sure that you do not shorten the textheight too much.

%%%%%%%%%%%%%%%%%%%%%%%%%%%%%%%%%%%%%%%%%%%%%%%%%%%%%%%%%%%%%%%%%%%%%%%%%%%%%%%%

%%%%%%%%%%%%%%%%%%%%%%%%%%%%%%%%%%%%%%%%%%%%%%%%%%%%%%%%%%%%%%%%%%%%%%%%%%%%%%%%

%%%%%%%%%%%%%%%%%%%%%%%%%%%%%%%%%%%%%%%%%%%%%%%%%%%%%%%%%%%%%%%%%%%%%%%%%%%%%%%%
\section*{APPENDIX}

Appendixes should appear before the acknowledgment.

\section*{ACKNOWLEDGMENT}

The preferred spelling of the word ÒacknowledgmentÓ in America is without an ÒeÓ after the ÒgÓ. Avoid the stilted expression, ÒOne of us (R. B. G.) thanks . . .Ó  Instead, try ÒR. B. G. thanksÓ. Put sponsor acknowledgments in the unnumbered footnote on the first page.

%%%%%%%%%%%%%%%%%%%%%%%%%%%%%%%%%%%%%%%%%%%%%%%%%%%%%%%%%%%%%%%%%%%%%%%%%%%%%%%%

References are important to the reader; therefore, each citation must be complete and correct. If at all possible, references should be commonly available publications.

\end{document}
